# Supplementary material for: Optimal Scalability-Aware Allocation of Swarm Robots: From Linear to Retrograde Performance via Marginal Gains
Source: arXiv:2512.23431 source file (2025-12-29)
Supplement: Supplementary file 1 [file supplementary_document.pdf]

# Optimal Scalability-Aware Allocation of Swarm Robots: From Linear to Retrograde Performance via Marginal Gains – Supplementary Document

Simay Atasoy Bingöl[1,2], Tobias Töpfer[1], Sven Kosub[1], Heiko Hamann[1,2], Andreagiovanni Reina[1,2,3]

[1]Department of Computer and Information Science, Universität Konstanz, Germany

[2]Centre for the Advanced Study of Collective Behaviour (CASCB), Universität Konstanz, Konstanz, Germany

[3]Department of Collective Behaviour, Max Planck Institute of Animal Behavior, Konstanz, Germany

## 1. EFFECT OF ARENA SIZE ON COLLECTIVE PERFORMANCE

We tested the influence of the arena size by repeating the simulations in the checkerboard environment with fill ratios $f \in \{0.51, 0.52, 0.53, 0.54, 0.55\}$ in a larger arena of $72 \times 72$ $su$. We conducted this analysis for both centralized and decentralized controllers and conducted 100 independent experiments for each fill ratio and controller. In the decentralized case, we doubled the communication radius to maintain a comparable relative range, since the arena side lengths were scaled by a factor of two (resulting in a fourfold increase in area).

The results for the larger arena are shown in Fig. S1. The trends in performance remain consistent across arena sizes for both controllers. The individual accuracy values $p$ are reported in Table S1.

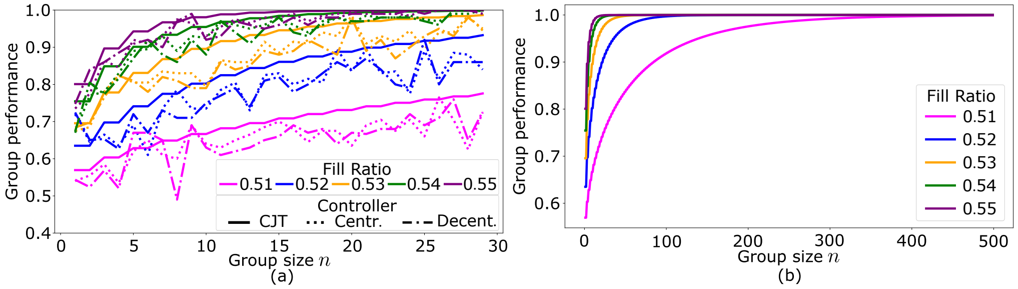


**Fig. S1.** In the larger checkerboard environment of size $72 \times 72$ $su$, scaling of the group accuracy (horizontal axis) in making majority decisions for different group sizes (vertical axis). The different colors show the results for different fill ratios. Solid lines show the CJT predictions and, in (a), the dotted and dashed lines show the multi-agent results for the centralized and decentralized controllers, respectively. In (b), the CJT lines are extended to larger swarm sizes, using the same values of individual accuracy probability $p$ as in (a) and in S1.

## 2. EXTENDED ENVIRONMENT ANALYSIS

### A. Fill Ratios

In the main text, we restricted our analysis to fill ratios in the range $0.51 \leq f \leq 0.55$ representing challenging tasks. We additionally performed experiments with larger fill ratios

**Table S1.** Individual Agent Accuracy for the Considered Environments

| arena size | 0.51 | 0.52 | 0.53 | 0.54 | 0.55 |
|---|---|---|---|---|---|
| $36 \times 36\ su$ | 0.5361 | 0.6017 | 0.6603 | 0.7454 | 0.8069 |
| $72 \times 72\ su$ | 0.5694 | 0.6350 | 0.6955 | 0.7545 | 0.8008 |

$f \in \{0.58, 0.60, 0.65\}$ representing easier tasks, and report the results in Fig. S2. The corresponding measured individual accuracy values are $p = \{0.8969, 0.9379, 0.9873\}$ for $f = \{0.58, 0.60, 0.65\}$, respectively. Because these values are approaching perfect accuracy $p = 1$, the experiments with larger fill ratios provide limited insight into task allocation. Instead, we focused on smaller fill ratios in our main analysis.

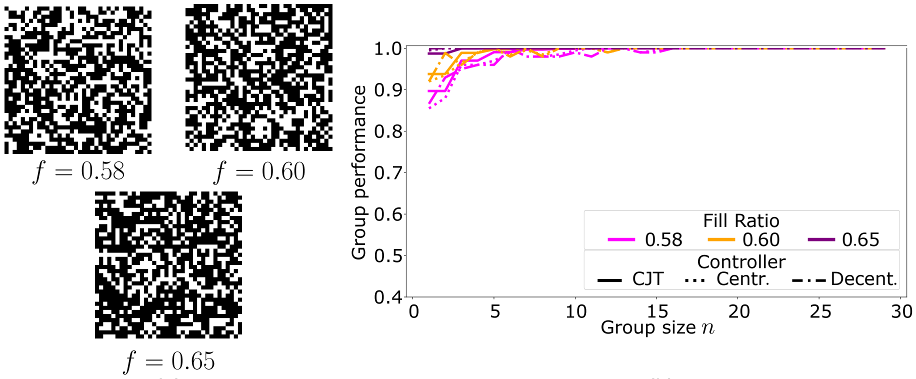


(a) (b)

**Fig. S2.** (a) Examples of checkerboard environments for the considered fill ratios. (b) Scaling of the group accuracy (vertical axis) in making majority decisions for different group sizes (horizontal axis) in the checkerboard environment for different fill ratios. The different colors show the fill ratios and the line types match the ones used in Fig. S1.

## B. Spatial Distributions

We further extended our analysis to additional spatial distributions of black and white tiles, namely the so-called *star* and *band-r* environments [1]. Consistent with our discussion in the main text, we keep the same fill ratio $f = 0.52$. The measured individual accuracy probabilities $p$ are 0.7189 and 0.8066 for star and band-r environments, respectively. The corresponding results are given in Fig. S3.

Based on our intuition, we would have expected the individual accuracy probability $p$ to follow the order: checkerboard, star, striped, four rectangles, band-r, and halved. However, the results turned out differently. The obtained accuracy $p$ also depends on the implementation of the random walk behavior of the agents. The effect is illustrated by the heatmap of agent locations in Fig. S3(c). The central area of the arena is rarely visited, which explains the relatively high $p$ value observed for the band-r environment.

# 3. ADDITIONAL TASK ALLOCATION RESULTS

In the main text, we primarily reported task allocation results for binary classification in environments with different fill ratios. Here, we additionally present results for three scenarios with varying spatial distributions. To maintain consistency with the main text, Fig. S4 shows the allocation outcomes for $N = 30$ (left column) and $N = 150$ (right column). As observed previously, increasing the swarm size shifts the optimal allocation towards the most difficult task(s).

An interesting observation arises in the first row of Fig. S4, where the striped, four rectangles, and halved environments are considered. The corresponding $p$ values for these three environments are relatively low compared to other environments. With only 150 agents, the swarm size is not sufficient to shift the allocation decisively toward the halved environment (the one with the

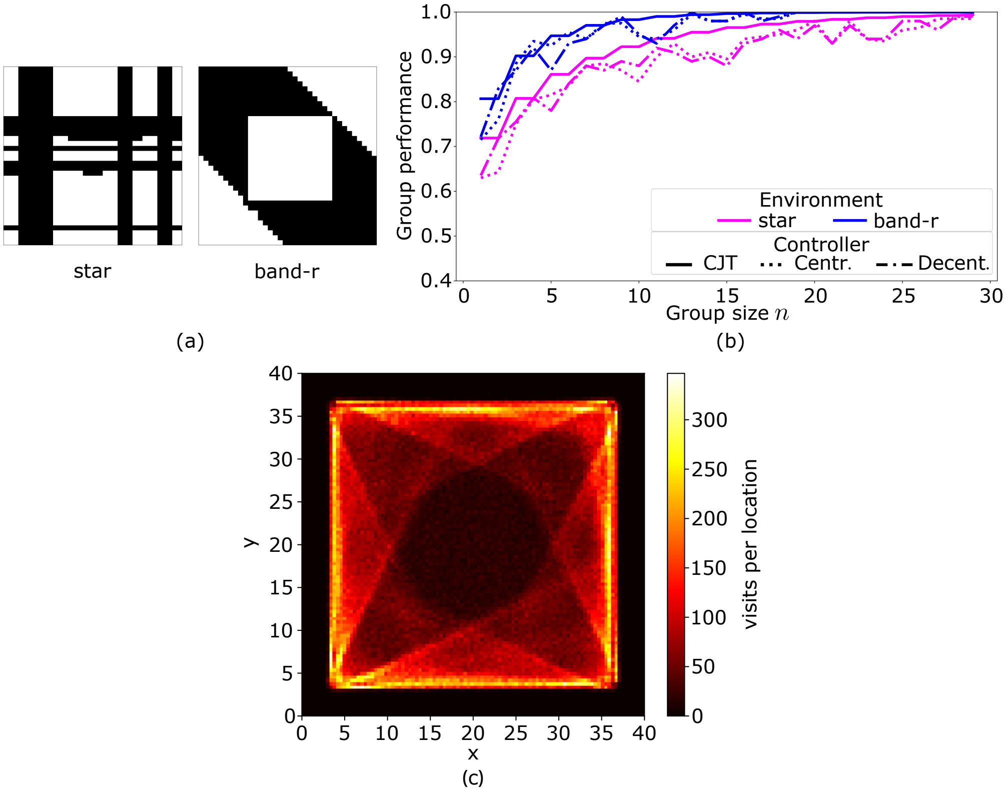


**Fig. S3.** (a) Illustration of star and band-r environments. (b) Scaling of the group accuracy (vertical axis) in making majority decisions for different group sizes (horizontal axis) in the star and band-r environments. The different colors show the different environments and the line types match the ones used in Fig. S1. (c) Histogram of agent positions aggregated over all experiments. The heatmap represents the visitation frequency of each location in the arena.

lowest $p$). Instead, the optimal allocation assigns more agents to the striped and four rectangles environments. This result indicates that when tasks have low performance, we may still allocate more agents to comparatively easier tasks for medium swarm sizes, and only at substantially larger swarm sizes, the allocation converges towards the task with the lowest $p$ (hardest task).

## REFERENCES

1. P. Bartashevich and S. Mostaghim, “Benchmarking collective perception: New task difficulty metrics for collective decision-making,” in *EPIA Conference on Artificial Intelligence*, (Springer, 2019), pp. 699–711.

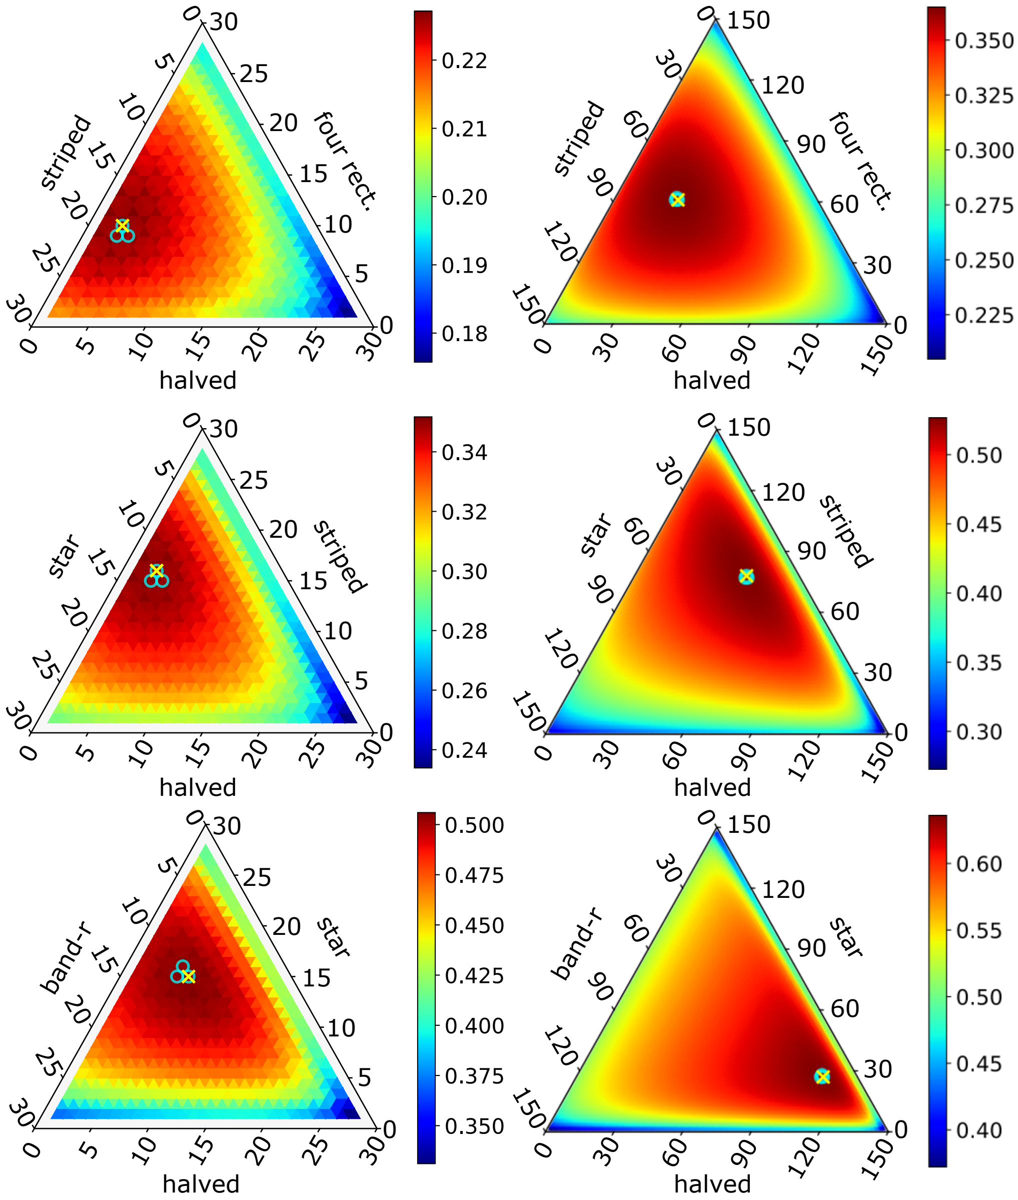


**Fig. S4.** Three scenarios for the allocation of agents to $T = 3$ collective decision-making tasks. Blue circles mark the agent allocation yielding the highest performance, while the yellow cross indicates the allocation computed by our algorithm, which always coincides with one of the blue circles.
